# Supplementary material for: Data and Representation for Turkish Natural Language Inference
Source: arXiv:2004.14963 source file (2020-10-20)
Supplement: Supplementary file 1 [file appendix_additional_details.tex]

\subsection*{Additional Experiment Details}
\label{sec:appendix-additional-details}

Additional experimentation details are available in Reproducibility-Notes.pdf inside our code files (turkish-nli-code.zip) that are uploaded into the upload system.
